# Supplementary material for: "If sighted people know, I should be able to know:" Privacy Perceptions of Bystanders with Visual Impairments around Camera-based Technology
Source: arXiv:2210.12232 source file (2022-10-21)
Supplement: Supplementary file 1 [file 8-appendix-2.tex]

% \clearpage
\newpage
\normalsize
\section{Additional Appendix}
\subsection{Survey Questions}
\subsubsection{Screening questions}
\begin{enumerate}
    \item[1.1] Are you visually impaired or sighted?
    \item[1.2] Are you above 18 years old?
\end{enumerate}

\subsubsection{Demographic Questions}
\textit{For visually impaired participants only:}
\begin{enumerate}
    \item[2.1] Are you legally blind?
    \item[2.2] Do you have functional vision?
    \item[2.3] What is your visual acuity?
    \item[2.4] What is your field of view?
\end{enumerate}
\textit{For all participants:}
\begin{enumerate}
    \item[2.5] How do you identify your gender?
    \item[2.6] What is your age?
\end{enumerate}

\subsubsection{Scenario-based Questions}
\textit{The survey included 12 scenarios as shown in Table \ref{tab:scenario}. We randomized the order of the scenarios presented to each participant. We repeated the same questions for each scenario:}
\begin{enumerate}
    \item[3.1] How comfortable would you feel in this scenario? (Extremely comfortable, Somewhat comfortable, Neutral, Somewhat uncomfortable, Extremely uncomfortable.)
%    \item[3.2] Can you briefly explain your selection about your comfort level?
    \item[3.2] In this scenario, would you be able to notice whether you or some of your information are captured by the camera? (I can always/ sometimes/ seldomly/ never detect whether people are capturing me.)
\end{enumerate}

\subsubsection{Contact Information}
We plan to schedule a follow-up interview via Zoom to have a deeper understanding of your perceptions of different scenarios. The interview will take around 1 hour and we will provide a \$15 visa card as a compensation for your time. If you are interested in participating in the interview study, please leave your name and phone number or email address.

\begin{enumerate}
    \item[4.1] What's your name?
    \item[4.2] What's your email address?
    \item[4.3] What's your phone number?
\end{enumerate}

%\section{Appendix for Study II}
\subsection{Interview Script}
\label{sec: interview}
\subsubsection{General Background Questions}
\begin{enumerate}
    \item[1.1] Please describe your visual ability?
        \begin{itemize}
            \item[1.1.1] Are you legally blind?
            \item[1.1.2] Do you have functional vision?
            \item[1.1.3] What is the diagnosis of your visual condition?
            \item[1.1.4] What is your visual acuity?
            \item[1.1.5] What is your field of view?
            \item[1.1.6] How is your light perception?
        \end{itemize}
    \item[1.2] What is your education level?
    \item[1.3] What assistive technology do you usually use in daily life? 
    \item[1.4] Do you live alone or do you live with your family?
    \item[1.5] Do you live in city or rural area? 
    \item[1.6] Are you familiar with the usages of cameras?
        \begin{itemize}
            \item[1.6.1] If yes, can you describe what camera-based technology do you use in daily life and how do you use them? 
            \item[1.6.2] If no, why?
        \end{itemize}
    \item[1.7] What do you think are the benefits of using camera-based technology?
    \item[1.8] What concerns do you have regarding the use of camera-based technology?
    \item[1.9] Have you ever had any experience where you were captured by other people’s cameras? Can you elaborate on your experience?
\end{enumerate}

\subsubsection{Scenario-based Questions}
\textit{The interview included four scenarios: a maintenance person uses a smartphone to take photos at your home (S2); your roommate uses smartglasses in the apartment (S5); a stranger using smartglasses in a public bathroom in a mall (S6); and a colleague sitting beside you sets up a security camera on his/her desk (S10), as shown in Table \ref{tab:scenario}. We randomized the order of the scenarios presented to each participant. We repeated the same questions for each scenario:}

\begin{itemize}
    \item[2.1] Have you encountered any similar scenario in your life? Can you describe it?
    \item[2.2] How comfortable would you feel when they have such behavior? We used a 5-point Likert scale (1: extremely uncomfortable, 5: extremely comfortable)?
    \item[2.3] Why do you give this score?
    \item[2.4] What information do you feel comfortable to be captured? And what information do you not feel comfortable to be captured in this scenario? 
    \item[2.5] Are you able to notice whether the particular camera is being used in this scenario? 
    
        \textit{If yes:}
        \begin{itemize}
            \item[2.5.1] How do you detect the use of the camera?
            \item[2.5.2] How effective do you feel your strategy is?  
        \end{itemize}
        
        \textit{If no:}
        \begin{itemize}
            \item[2.5.3]
            \item[2.5.4] How important is this information to you? 
            \item[2.5.5] How do you feel about not being able to detect the camera in this scenario? 
        \end{itemize}
    \item[2.6] Are you able to detect whether you are in the coverage of their camera?
    
        \textit{If yes:}
        \begin{itemize}
            \item[2.6.1] How do you detect the use of the camera?
            \item[2.6.2] How effective do you feel your strategy is?  
        \end{itemize}
        
        \textit{If no:}
        \begin{itemize}
            \item[2.6.3] Are you willing to detect whether they are capturing you? 
            \item[2.6.4] How important is this information to you? 
            \item[2.6.5] How do you feel about not being able to detect whether you or your information is being captured in this scenario? 
        \end{itemize}
        
    \item[2.7] Are you able to avoid being captured by their camera?
    
        \textit{If yes:}
        \begin{itemize}
            \item[2.7.1] How do you detect the use of the camera?
            \item[2.7.2] How effective do you feel your strategy is?  
        \end{itemize}
        
        \textit{If no:}
        \begin{itemize}
            \item[2.7.3] Are you willing to detect whether they are capturing you? 
            \item[2.7.4] How important is this information to you? 
            \item[2.7.5] How do you feel about not being able to avoid being captured in this scenario? 
        \end{itemize}
        
    \item[2.8] Will you communicate your concerns and preferences with the technology user in this scenario? 
        \begin{itemize}
            \item[2.8.1] If yes, how would you communicate your preference with the technology user?
            \item[2.8.2] If no, why?
        \end{itemize}
     
    \item[2.9] What do you think the photos taken in this scenario would be used for? 
        \begin{itemize}
            \item[2.9.1] Who would you think would be able to access these photos?
            \item[2.9.2] How comfortable are you with such use of the photos of you or your information?
            \item[2.9.3] If you don’t feel comfortable, what strategy would you use to protect yourself?
            \item[2.9.4] How effective do you feel this strategy is?  
            \item[2.9.5] How important is this information control to you? 
            \item[2.9.6] How do you feel about not being able to control the use of the photos with you or your information? 
        \end{itemize}
        
\end{itemize}

\subsubsection{Technology Design Questions}
\begin{itemize}
    \item[3.1] In general, how comfortable do you feel if there are cameras use around you?
    \item[3.2] Will different types of cameras make a difference for your privacy perception? Why?
    \item[3.3] Will the location, public vs private, make a difference for you? Why?
    \item[3.4] Will the owners of the camera, stranger or acquaintance, make a difference for you? Why?
    \item[3.5] How comfortable do you feel if the user of the camera has visual impairments?
    \item[3.6] What information do you consider as private information that you do not want others to capture, even accidentally?
    \item[3.7] Besides the scenarios we’ve discussed above, is there any other scenarios in your real-life where you had concerns about as a bystander of sensing technology? Can you elaborate on it?
   % \item[3.8] Did you communicate your concerns and preferences with the technology user? How did you communicate your preference with the technology user?
    \item[3.8] When there are cameras being used around you, what information do you want to know about these cameras? 
    \item[3.9] What would be your preferred way to get such information?
    \item[3.10] Imagine that you can design any technology to notify you of the camera use nearby and protect your privacy, how do you want this technology to look like?
        \begin{itemize}
            \item[3.10.1] What device or platform do you prefer?
            \item[3.10.2] What feedback do you prefer for camera awareness?
            \item[3.10.3] What interactions do you prefer to better control other people' access to your information? %How do you want to control what types of your information other people are able to capture via the camera?
        \end{itemize}
\end{itemize}

\subsection{Codebook and Themes}

\begin{table*}
  \centering
  \setlength{\tabcolsep}{2.5pt}
  % \renewcommand{\arraystretch}{1.2}
  % \resizebox{\textwidth}{!}{%
      \small
    \begin{tabular}{m{10em}     % themes
                    m{15em}     % subthemes 
                    m{25em}}      % codes
    &&&
   % \multicolumn{4}{c}{\textbf{Deployability}} &
   % \multicolumn{7}{c}{\textbf{Usability}} &
   % \multicolumn{5}{c}{\textbf{Accessibility}} &
   % \multicolumn{4}{c}{\textbf{Security}} \\
   % \cmidrule{5-24}
    \textbf{Themes}& \textbf{Sub-themes} & \textbf{Codes}\\
    \midrule
    %
    %%%%%%%%%%%%%%%%%%%%%%%%%%
    % PHYSICAL BIOMETRICS
    %%%%%%%%%%%%%%%%%%%%%%%%%%
    %
    \multirow{13}{10em}{No Agency to Detect/Avoid Cameras} 
    &  
    No access to camera info  & unable to detect; camera presence; camera location; camera range; unable to avoid; no control; frustrating; lack of agency\\ 
    \cline{2-3}
    &
    Passively infer camera usage  & audio cues; shutter sound; audio cue not effective; audio muted; hard to hear; hard to distinguish source; overhear conversation; notified by others; do not expect cam user to inform; hard to form privacy opinion \\ 
    \cline{2-3}
    &
    Communication to protect privacy  & communicate with cam user; ask for info; negotiate for agreement; confront; withdraw oneself; resignation; avoidance; unable to communicate; unwilling to communicate; information uncertainty; confirm camera users' behaviors; no control \\ 
    \cline{2-3}
    &
    Unique challenges of low vision & visual cues; light indicator; smartglasses vs normal glasses; body language of using camera; small; invisible; wearable camera harder to see \\
    \midrule
    \multirow{8}{10em}{Adapted Privacy Perceptions} 
    &  
    Common perception  & public camera; public place; uncomfortable with personal camera; intentional; uncomfortable with private place; disguised cam; malicious purpose; compromise to social norms; uncomfortable at first; get used to cam; \\ 
    \cline{2-3}
    &
    Low privacy expectation  & low privacy expectation; self-regulation; expect no privacy; assume camera everywhere; no concerns; self-blame; put sensitive info away;   \\ 
    \cline{2-3}
    &
    High trust on acquaintances  & trust acquaintances; assume harmless purpose; easy to communicate with acquaintances; more likely be informed; willing to accommodate; cautious about strangers; check photos \\ 
    \midrule
    \multirow{8}{10em}{Empathy towards Camera Users with Disabilities} 
    &  
    High tolerance towards \newline camera-based assistive tech  & own experience of camera-based assistive tech; smartglasses as assistive tech; clear purpose; empathy; navigation; assistance; Aria \\ 
    \cline{2-3}
    &
    Tolerance to an extent  & no camera-based assistive tech at sensitive location; no 24/7 use; familiar place; no need to use; understand but not comfortable; confirm usage for assistive purpose; privacy policy of camera-based assistive tech \\ 
    \cline{2-3}
    &
    No additional tolerance  & no empathy; no difference from others; PVI can use camera for malicious purpose; judge based on one's own experience  \\ 
    \midrule
     \multirow{8}{10em}{Complication in a Sighted World} 
    &  
    Privacy inequity between \newline BVI and sighted people & unfair; unequal information access as bystander; unequal info exchange; desire for equal access; PVI use camera with screen reader;   \\ 
    \cline{2-3}
    &
    Privacy not respected by \newline sighted people  & guide dog attract camera; become camera target; photo taken without notification \\ 
    \cline{2-3}
    &
    Weight others' privacy more  & sighed bystanders; other bystanders; sighted remote agent; worry about others' privacy \\
    \cline{2-3}
    &
    Hope for understanding \newline from sighted people  & importance of camera-based assistive tech; sighted people not understand; right to use camera as assistive tech; desire for understanding; proper communication for education; camera-based assistive tech as accepted norm \\ 
    \midrule
    \multirow{8}{10em}{Expected Privacy Enhancements} 
    &  
    Info transparency and certainty & transparency of camera use; courtesy; information certainty; expected camera info; camera presence; camera range; camera purpose; whether oneself in camera; photo propagation; camera user; device type; camera location; modality of recorded info\\ 
    \cline{2-3}
    &
    Consent  & ask for consent \\ 
    \cline{2-3}
    &
    Desired privacy-enhancing tech  & necessity of privacy-enhancing tech; form factor; smartphone; smartwatch; necklace; wristband; audio feedback; haptic feedback; unobtrusive; proactive notification; pressure on users; low cost \\
    \cline{2-3}
    &
    Camera regulation policy \newline from sighted people  & workspace policy; policy by camera company; forced shutter sound\\ 
   
    \midrule
    \end{tabular}
%  }
    \caption{Themes and codebook in Study II.}
    \label{tab:codebook}
\end{figure*}

%%% Local Variables:
%%% mode: latex
%%% TeX-master: "../main"
%%% End:
