# Supplementary material for: "If sighted people know, I should be able to know:" Privacy Perceptions of Bystanders with Visual Impairments around Camera-based Technology
Source: arXiv:2210.12232 source file (2022-10-21)
Supplement: Supplementary file 2 [file tab_demographics_appendix.tex]

\begin{figure}[h]
  \centering\gamesfontsize
  \resizebox{0.4\textwidth}{!}{
  \begin{tabular}{lrr}
    \toprule
    Demographic item & N & \% \\
    \midrule
    Total & 90 & \\
    \midrule
    \textbf{Age} &&\\
    18-24 & 55 & 39.6 \\
    25-34 & 33 & 23.7 \\
    35-44 & 35 & 25.2 \\
    45-54 & 11 & 7.9 \\
    55-64 & 3 & 2.2 \\
    More than 65 yrs. & 2 & 1.4 \\
    \midrule
    \textbf{Gender} &&\\
    Female & 56 & 5.8\\
    Male & 32 & 91.4\\ 
    Prefer not to disclose & 1 & 2.2\\
    Prefer to self-describe & 1 & 0.7\\
    \bottomrule
  \end{tabular}}
  \caption{Summary of participant demographics.}
  \label{tab:demographics}
\end{figure}
